# Supplementary material for: Monitoring of Perception Systems: Deterministic, Probabilistic, and Learning-based Fault Detection and Identification
Source: arXiv:2205.10906 source file (2022-05-22)
Supplement: Supplementary file 1 [file appendix-SVM.tex]

%!TEX root = ../../main.tex

%%%%%%%%%%%%%%%%%%%%%%%%%%%%%%%%%%%%%%%%%%%%%%%%%%%%%%%%%%%%%%%%%%%%%%%%%%%%%%%%%%
\subsubsection{Learning the Factor Graph Parameters}\label{sec:training_fg}

This section discusses how to estimate parameters that determine factors in a factor graph from 
a given training dataset.
In particular, review a method called \emph{structured support vector machine (SVM)} or \emph{maximum margin learning}~\cite{Murphy12book-MLProbabilisticPerspective}.

The idea of SVM is to train a function with good predictive qualities by minimizing the expected risk, namely
\begin{equation*}
  \argmin_\faults \sum_{\faults^\prime} \loss(\faults,\faults^\prime) \marginal(\faults\mid\syndrome,\fgparams)
\end{equation*}
where $\loss(\faults,\faults^\prime)$ is the cost of predicting $\faults$ instead of $\faults^\prime$.
By including the loss function in the training we perform a ``loss-calibrated MAP parameter estimation''.
We can write the expected loss as \LC{unclear how you get here (also: you need to define $\fgparams$)}
\begin{equation*}
  R_{\mathrm{EL}} \triangleq -\log \marginal(\fgparams) + \sum_{(\faults,\syndrome)\sim\dataset} \log \left(
    \loss(\faults^\prime, \faults) \marginal(\faults\mid\syndrome,\fgparams)
  \right)
\end{equation*}
Note that we can rewrite \cref{eq:factor_graph} as: \LC{also this requires a bit more explanation}
\begin{equation*}
  \marginal(\faults\mid\syndrome,\fgparams) = \frac{\exp(\fgparams\tran \featuremap(\faults,\syndrome))}{\partitionfcn(\faults, \fgparams)}
\end{equation*}
\red{still hard to follow:
The \emph{feature map} $\featuremap(\faults,\syndrome)$ is a function that maps the input and outputs of the model to a space used by the inner product.
The feature maps are implicitly specified by the factor graph and its parameterization, and they simply select the right element of the parameters vector $\fgparams$ for the specific configuration $(\faults, \syndromevar)$.
It can be proven~\cite{Murphy12book-MLProbabilisticPerspective} that the expected loss $R_{\mathrm{El}}$ is upper bounded by
\begin{equation*}
  R_{\mathrm{EL}} \leq E(\fgparams) + \sum_{(\faults,\syndrome)\sim\dataset} \left( 
    \max_{\faults^\prime} \left( \logloss(\faults, \faults^\prime) + \fgparams\tran\featuremap(\faults^\prime,\syndrome) \right) - \fgparams\tran\featuremap(\faults,\syndrome)
    \right)
\end{equation*}
Where we took $\logloss(\faults^\prime,\faults) =  \log\loss(\faults^\prime,\faults)$ and $\marginal(\fgparams)=\exp(-E(\fgparams))/Z$ for an appropriate energy potential $E$.
If we set $E(\fgparams) = \frac{1}{2C}\|\fgparams\|_2^2$, corresponding to a spherical Gaussian prior we obtain we obtain
\begin{equation}\label{eq:regularized_empirical_risk}
  R_{\mathrm{SSVM}} \triangleq \frac{1}{2}\|\fgparams\|_2^2 + C\sum_{(\faults,\syndrome)\sim\dataset} \left( 
    \max_{\faults^\prime} \left( \logloss(\faults, \faults^\prime) + \fgparams\tran\featuremap(\faults^\prime,\syndrome) \right) - \fgparams\tran\featuremap(\faults,\syndrome)
    \right)
\end{equation}

Optimize \cref{eq:regularized_empirical_risk} is difficult in general, however it has been shown that it is sufficient to minimize a convex upper bound.
A common way to find the optimal parameters is to solve a problem called \emph{loss augmentation}, which consist in solving
\begin{equation}\label{eq:loss_augmentation}
\fgparams^* = \argmin_{\fgparams} \; \frac{1}{2}\|\fgparams\|^2 + \frac{\lambda}{|\dataset|} \sum_{(\faults,\syndrome)\in\dataset}\ell(\faults,\syndrome, \fgparams)  
\end{equation}
with
\begin{equation}
% \ell(\faults,\syndrome,\fgparams) = \max_{\syndrome^\prime} \left( \loss(\syndrome,\syndrome^\prime) - g(\faults,\syndrome,\fgparams) + g(\faults,\syndrome^\prime,\fgparams) \right)
\ell(\faults,\syndrome,\fgparams) = \max_{\faults^\prime} \left( \logloss(\faults, \faults^\prime) + \fgparams\tran\featuremap(\faults^\prime,\syndrome) \right) - \fgparams\tran\featuremap(\faults,\syndrome)
\end{equation}
% \cref{eq:loss_augmentation} is derived from \cref{eq:regularized_empirical_risk} by choosing $r=1/2 \|\fgparams\|^2$ and replacing $\loss$ with its upper bound $\ell$.
\cref{eq:loss_augmentation} is derived from \cref{eq:regularized_empirical_risk} by replacing $\loss$ with its upper bound $\ell$.
To show that $\ell$ is indeed an upper bound,
given a syndrome $\syndrome$, let $\faults^* = \argmax_\faults \fgparams\tran\featuremap(\faults,\syndrome)$, we have
\begin{align*}
  \logloss(\faults,\faults^*) 
    &\leq \logloss(\faults, \faults^*) + \fgparams\tran\featuremap(\faults^*,\syndrome) - \fgparams\tran\featuremap(\faults,\syndrome)  \\
    &\leq \max_{\faults^\prime} \left( \logloss(\faults,\faults^\prime) + \fgparams\tran\featuremap(\faults^\prime,\syndrome) \right) - \fgparams\tran\featuremap(\faults,\syndrome)\\
    &= \ell(\faults,\syndrome,\fgparams)
\end{align*}
% Rewriting the log-factors as
% \begin{equation*}
  % \log \factorvar (\faults;\syndrome,\fgparams) = \logfactor(\syndrome\;\faults,\fgparams) = \langle \fgparams, \featuremap_\factorvar \rangle
% \end{equation*}
% Here the feature map or sufficient statistics $\featuremap$ of the model denotes a mapping from the input and output domain to a joint input/output space.
% The linearity of the energy in the parameters simplifies the estimation of $\fgparams$ considerably.
It easy to show that $\ell$ is convex because is the maximum over many functions that are affine in $\fgparams$.

Since loss augmentation problem in \cref{eq:loss_augmentation} is convex, we can standard convex optimization methods to find its global minimum.
}
