# Supplementary material for: Monitoring of Perception Systems: Deterministic, Probabilistic, and Learning-based Fault Detection and Identification
Source: arXiv:2205.10906 source file (2022-05-22)
Supplement: Supplementary file 2 [file appendix-bp.tex]

%!TEX root = ../../main.tex

\section{Appendix: Belief Propagation}\label{sec:belief_propagation}

\red{
In this section, we discuss a popular method for inference on discrete factor graphs.

% \subsubsection{From \DGraphs to Factor Graphs
% \subsubsection{Belief Propagation}\label{sec:belief_propagation}

The \emph{belief propagation} (also known as sum-product algorithm) is a dynamic programming algorithm that, given a factorization in the form \cref{eq:factor_graph}, computes the marginal distributions for all the variables $v\in\varset$ and factors $\factorvar\in\factorset$.
The algorithm was initially developed for tree-structured factor graphs (graphs that are connected and do not contain cycles), however, it can be modified to work on general factor graphs, in which case we refer to it as \emph{loopy belief propagation}.
We will describe the algorithm in terms of log-factors. 
%we re-parametrize each factor into log-space.
For a factor $\factorvar_i\in\factorset$ we set 
\begin{equation}\label{eq:log_factor}
  \logfactor_i(\vy_{\neighbors(\factorvar_i)})=\log(\factorvar_i(\vy_{\neighbors(\factorvar_i)}))
\end{equation}
The algorithm is based on the computation of \emph{messages}.
For each edge $(v,\factorvar)\in\fgedgeset$, it defines a \emph{variable-to-factor} message
$q_{v\to\factorvar}:\dom(i)\to\Reals{}$ 
and a \emph{factor-to-variable} message
$r_{\factorvar\to v}:\dom(v)\to\Reals{}$.
For computing the variable-to-factor message, consider the set of factors adjacent to a variable $v$ as $\neighbors(v)$ (recall that the factor graph is a bipartite graph so the neighbors of a node are factors and vice versa),
then, the message is computed as
\begin{equation}\label{eq:variable_to_factor_message}
  q_{v\to\factorvar}(y_v) = 
  \sum_{\factorvar^\prime\in\neighbors(v)\setminus\{\factorvar\}} 
  r_{\factorvar^\prime\to v}(y_v)
\end{equation}
with the convention that, if there is no term in the summation, the message is simply zero.
For the factor-to-variable message instead
\begin{equation}\label{eq:factor_to_variable_message}
  r_{\factorvar\to i}(y_v) = \log
  \sum_{\vy^\prime : y^\prime_v=y_v}\exp\left( 
    -\logfactor_\factorvar(\vy^\prime_{\neighbors(\factorvar)}) + 
    \sum_{u\in\neighbors(\factorvar)\setminus\{v\}} \vq_{u\to\factorvar}(y_u)
  \right) 
\end{equation}
\cref{eq:variable_to_factor_message,,eq:factor_to_variable_message} depend on previously computed messages.
For tree-structured factor graphs, there always exists at least one leaf node where the initial message can be computed.
To compute all the messages we first chose an arbitrary node as root, say $v_k$, then we compute all messages directed towards the root, starting from the leaf nodes (because we know how to compute their messages).
Once we reach the root, we reverse the schedule computing all messages moving away from the root.
When this second phase is complete, we have computed all messages.

The value of the partition function $\partitionfcn$ can be computed by summing all factor-to-variable messages directed to the tree root $v_k$
\begin{equation}
  \log \partitionfcn = 
  \log \sum_{y_k} \exp \left( \sum_{\factorvar\in\neighbors(v_k)} r_{\factorvar\to v_k} (y_k)\right)
\end{equation}
At this point, we can compute both the factors' marginals and the variable marginals.
For a factor
\begin{equation}
\marginal(Y_{\neighbors(\factorvar)}=\vy_{\neighbors(\factorvar)}) = \exp\left(
    -\logfactor_\factorvar(\vy_{\neighbors(\factorvar)}) +
    \sum_{u\in\neighbors(\factorvar)} q_{u\to\factorvar}(y_u)
  \right)
\end{equation}
conversely, the variable marginals are computed as
\begin{equation}
  \marginal(Y_v=y_v) = \exp \left( 
    \sum_{\factorvar\in\neighbors(v)} r_{\factorvar\to v} (y_v) - \log \partitionfcn
  \right)
\end{equation}

\myParagraph{Loopy Belief Propagation}
When the factor graph is not tree-structured, the belief propagation algorithm is not applicable as we described above, as it is not possible to identify a leaf node.
In this case, we need to use a variation called \emph{loopy belief propagation}.
In the \emph{loopy belief propagation}, all messages are initialized to a fix value, and factor-to-variable messages $r_{\factorvar\to v}$ are computed as before.
The variable-to-factor messages, the marginals and the partition functions instead are normalized in every iteration.
The details of the method is \LC{beyond the scope of this paper}, for the interested reader, please refer to~\cite{Murphy12book-MLProbabilisticPerspective}.
Loopy Belief Propagation, it is not guaranteed to converge, however it is now known that if the algorithm converges, then it converged to a fix-point of the Bethe free energy~\cite{Nowozin11-structuredLearning}.
This property, together wth good empirical performances, make this algorithm a popular choice for approximate inference algorithm for discrete graphical models.

\myParagraph{Maximum a posteriori inference}\label{sec:max_product_alg}
The belief propagation algorithm can also be used to perform MAP inference.
As for probabilistic inference, it provides the exact solution in the case of tree-structured factor graphs, otherwise, it provides an approximation.
The MAP inference version of belief propagation is also known as \emph{max-product algorithm}, in the case of energies (like in this paper), is known as \emph{max-sum algorithm}.
The basic idea to enable MAP queries is to replace the marginalization operation performed in \cref{eq:factor_to_variable_message} by a maximization operation, becoming
\begin{equation}\label{eq:max_factor_to_variable_message}
  \vr_{\factorvar\to v}(y_v) = \max\left( 
    -\logfactor_\factorvar(\vy^\prime_{\neighbors(\factorvar)}) + 
    \sum_{u\in\neighbors(\factorvar)\setminus\{v\}} \vq_{u\to\factorvar}(y_u)
  \right) 
\end{equation}
Now the `max-beliefs' are no longer interpretable as marginals but instead they describes the maximum negative energy achievable when fixing the variable $v$ to $y_v$
\begin{equation*}
  \marginal_v(y_v) = \sum_{\factorvar^\prime\in\neighbors(v)} \vr_{\factorvar^\prime\to v}(y_v)
\end{equation*}
To recover a joint minimum energy configuration, we set each variable $v$ to the state attaining the maximum max-belief
\begin{equation*}
  y^*_v = \argmax_{y_v} \marginal_{\factorvar\to v}(y_v)
\end{equation*}
Belief propagation and the variation used for MAP inference only change in the message updates.
}
